# Supplementary material for: Fragile dislocation modes in obstructed atomic topological phases
Source: arXiv:2310.10779 ancillary file (2024-05-14)
Supplement: Supplementary file 1 [file SM.pdf]

# Supplemental Material: Fragile dislocation modes in obstructed atomic topological phases

Gabriel Malavé,[1] Jorge Schifferli,[2] Rodrigo Soto-Garrido,[1] Pedro A. Orellana,[2] and Vladimir Juričić[2,3]

[1] *Facultad de Física, Pontificia Universidad Católica de Chile, Vicuña Mackenna 4860, Santiago 8331150, Chile*

[2] *Departamento de Física, Universidad Técnica Federico Santa María, Casilla 110, Valparaíso, Chile*

[3] *Nordita, KTH Royal Institute of Technology and Stockholm University, Hannes Alfvéns väg 12, SE-106 91 Stockholm, Sweden*

The Supplemental Material contains: The details of the model and the analysis of the band structure in a defect-free system [Sec. S1]; The analysis of the symmetry of the trench modes [Sec. S2]; The details of the evolution of the fragile dislocation modes in the topological phase [Sec. S3]; The details of the evolution of the corner modes in the topological phase [Sec. S4].

## S1. BAND STRUCTURE OF THE DEFECT-FREE SYSTEM

We here present the spectrum of the two-dimensional (2D) Su-Schrieffer-Heeger (SSH) model, given by Eq.(1) in the main text, for completeness, $\hat{H} = \sum_{\mathbf{k}} \Psi_{\mathbf{k}}^{\dagger} \mathbb{H}_{\mathbf{k}} \Psi_{\mathbf{k}}$, with

$$\mathbb{H}_{\mathbf{k}} = \begin{pmatrix} 0 & \mathbb{Q} \\ \mathbb{Q}^{\dagger} & 0 \end{pmatrix}, \mathbb{Q} = \begin{pmatrix} t + \tau e^{2iak_x} & t + \tau e^{2iak_y} \\ t + \tau e^{-2iak_y} & t + \tau e^{-2iak_x} \end{pmatrix}, \tag{S1}$$

where $\Psi_{\mathbf{k}} = (c_{1,\mathbf{k}}, c_{2,\mathbf{k}}, c_{3,\mathbf{k}}, c_{4,\mathbf{k}})^{\top}$ represents the annihilation operator for the four sites in the unit cell, as shown in Fig. 1(a) in the main text, $c_{\alpha,\mathbf{k}}$, $\alpha = 1, ..., 4$ is the operator annihilating the state at the site $\alpha$ within the unit cell, with the momentum $\mathbf{k}$, and parameter $\tau$ $(t)$ represents the inter- (intra-)unit-cell hopping amplitude [1]. We then implement this Hamiltonian in the real space using Kwant code [2]. The above Hamiltonian can be cast in a more convenient form

$$\mathbb{H}_{\mathbf{k}} = \sum_{ij=0}^{3} A_{ij} \sigma_i \otimes \sigma_j, \tag{S2}$$

where the nonvanishing coefficients are

$$A_{10} = t + \tau \cos(2k_x a), \; A_{11} = t + \tau \cos(2k_y a), \; A_{23} = -\tau \sin(2k_x a), \; A_{12} = -\tau \sin(2k_y a). \tag{S3}$$

Here, $\sigma_0$ is the $2 \times 2$ identity matrix, and $\sigma_i$ $(i = 1, 2, 3)$ are the usual Pauli matrices. The corresponding spectrum features four bands of the form

$$E_{\alpha,\beta}(\mathbf{k}) = \alpha \sqrt{A_{10}^2 + A_{11}^2 + A_{23}^2 + A_{12}^2 + 2\beta \sqrt{(A_{10}^2 + A_{23}^2)(A_{11}^2 + A_{12}^2)}} \tag{S4}$$

$$= \alpha \sqrt{2} \sqrt{t^2 + \tau^2 + t\tau[\cos(2k_x a) + \cos(2k_y a)] + \beta \sqrt{[t^2 + \tau^2 + 2t\tau \cos(2k_x a)][t^2 + \tau^2 + 2t\tau \cos(2k_y a)]}}, \tag{S5}$$

where $\alpha, \beta = \pm$.

This Hamiltonian possesses $C_{4v}$ point-group symmetry, and as a consequence, the spatial inversion around the center of the unit cell, represented by $\mathcal{I}_S = \sigma_1 \otimes \sigma_0$. Furthermore, the model is time-reversal symmetric, with the time-reversal operator represented by $\mathcal{I}_T = K$, and $K$ as the complex conjugation, as can be explicitly checked in Eq. (S1). The bands with opposite sign of the energy, $E_{-,\beta} = -E_{+,\beta}$, are related by the chiral (unitary particle-hole) symmetry, which is represented by the operator $\Pi = \sigma_3 \otimes \sigma_0$, $\{\Pi, \mathbb{H}_{\mathbf{k}}\} = 0$. The zero-energy states, located along the diagonals $k_y = \pm k_x$ because of the two diagonal mirror symmetries, are doubly degenerate, as can be explicitly seen from the band structure in Eq. (S4), implying that they transform under the $E$ irreducible representation (irrep) of the $C_{4v}$ symmetry. All other finite energy states transform under either $A_1$ or $B_2$ one-dimensional (1D) irreducible representation of the $C_{4v}$ group at the high-symmetry $\Gamma = (0, 0)$ and the $M = (\pi, \pi)/2a$ points in the BZ. The

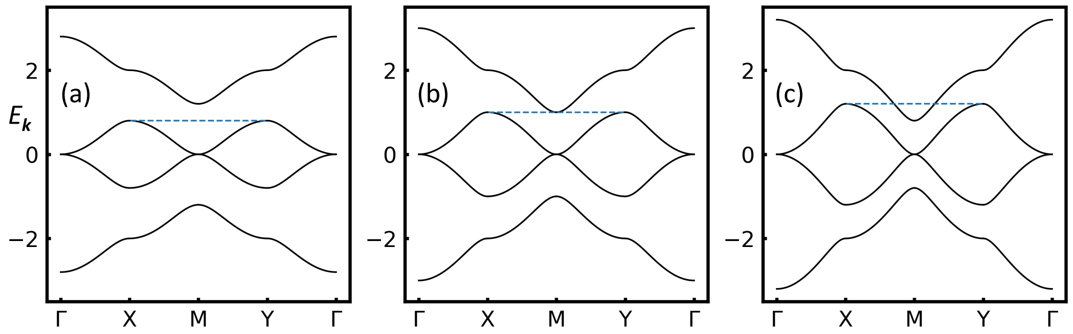


Figure S1. Bulk energy bands in the two-dimensional Su-Schrieffer-Heeger model given by Eq. (S1) for (a) $t = 0.4$, (b) $t = 0.5$, (c) $t = 0.6$. We here fix $\tau = 1$, and the blue dashed line connects the two minima of the lower positive-energy band. Therefore, the indirect gap is open in (a), at the closing point in (b), and closed in (c).

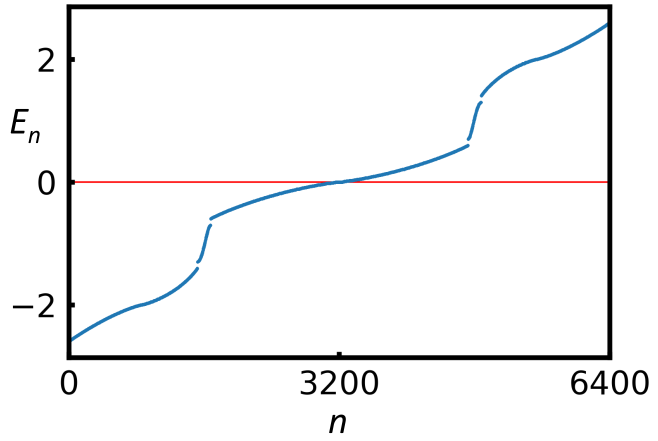


Figure S2. The spectrum of the 2D SSH model [Eq. (S1)] without the defect. We set $t = 0.3$ and $\tau = 1$. The system size is $40 \times 40$ unit cells, and open boundary conditions are employed. The reference energy $E = 0$ is marked by red line.

topological (trivial) phase is realized for $|t/\tau| < 1$ ($|t/\tau| > 1$), while phase transition occurs for $|t/\tau| = 1$, which is accompanied by a double band inversion: (i) at the $M$ point with the highest positive energy band inverting the irrep from $A_1$ (topological phase) to $B_2$ (trivial phase), and the lowest energy negative band from $B_2$ (topological phase) to $A_1$ (trivial phase); (ii) A band inversion at the $X$ and $Y$ points, which are invariant under the $C_{2v}$ subgroup of the full symmetry group $C_{4v}$ [3].

The forms of the band structure for various values of the parameters $t$ and $\tau = 1$ fixed are shown in Fig. S1. Importantly, the band structure features an *indirect* gap between the two bands with positive (negative) energies. The minimum of the band $E_{+,+}$ is at the $M$ point of the BZ at $(\pi, \pi)/2a$ with value $E_{+,+}(\pi/2a, \pi/2a) = 2|t-\tau|$, while the maximum of the band $E_{+,-}$ is at the symmetry related $X$ and $Y$ points, $E_{+,-}(0, \pi/2a) = E_{+,-}(\pi/2a, 0) = 2|t|$, when $|t/\tau| < 1$ (topological phase). Therefore, indirect bandgap is $\delta E_{\rm ind} = 2|\tau| - 4|t|$. The gap opens in the topological phase, but only in the region for $|t/\tau| < 0.5$, which, as shown in the main text, is the region where the dislocation modes are stable. The spectrum of the defect-free system in the topological regime ($t = 0.3$) in Fig. S2, shows that indirect gap between the closest-to-zero-energy states and the highest energy positive band (in the periodic system) is occupied by the band of the (finite energy) states, which are localized at the edge (localization is not explicitly shown here). On the other hand, when for $0.5 < |t/\tau| < 1$, the indirect gap closes, and the edge states become degenerate in energy with (some of) the bulk ones.

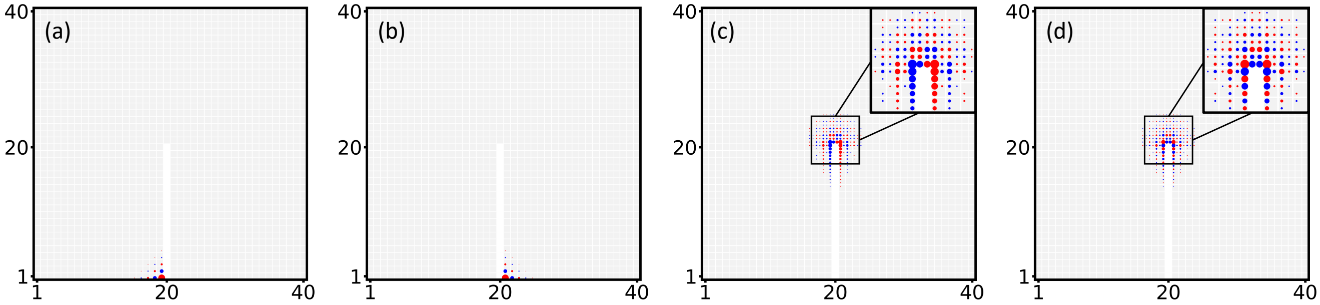


Figure S3. Low-energy modes at the sides of the trench formed before the edges are reconnected across the removed line of unit cells. Two zero-energy modes are localized at the lower (a) left and (b) right corners of the trench. Two finite-energy modes at (c) $E = 1.33$ and (d) $E = -1.33$ are localized at the upper corners of the trench and transform under $B$ and $A$ irreducible representations of the $C_2$ group, respectively. The values of the parameters are identical to Fig. S2. As in Fig. 2 of the Main Text, the red (blue) color denotes the positive (negative) phase of the wavefunction $\Psi_i$, while the point area is proportional to the amplitude $|\Psi_i|$ at the lattice site $i$. The zoom-in of each mode is shown in the inset of panels (c) and (d). Sites with an amplitude value less than $10^{-2}$ are left empty.

## S2. TRENCH MODES

To elucidate the origin of the dislocation modes, we here discuss the form and symmetry content of the modes localized at the trenches. These are formed in the Volterra construction of a dislocation defect after a line of unit cells is removed from the lattice and before the bonds across the trench are reconnected. The lattice symmetry, in this case, reduces to $C_2$, because of the cut introduced by the removal of a line of unit cells. The lattice recovers its full $C_{4v}$ symmetry only after the bonds across the trench are reconnected. The trench consists of four corners, which are, however, inequivalent. The lower corners are disconnected and therefore host two zero energy modes, as shown in Fig. S3(a) and (b). On the other hand, the two upper corners are connected, and therefore the would-be zero modes hybridize, yielding a pair of symmetrically split finite-energy modes, which transform under $B$ and $A$ representations of the $C_2$ group, shown, respectively, in Fig. S3(c) and (d). After the dislocation is formed by introducing the bonds across the trench, the two zero energy at lower corners hybridize and symmetrically split about zero energy. Furthermore, they localize at the defect core because of the effective $\pi$-flux sourced by the dislocation [4], and thus form a chiral pair of $A_1$ and $B_2$ modes. The finite-energy modes at the upper corner, upon the increase of symmetry, also localize and organize into a chiral pair of $A_1$ and $B_2$ modes, with the real-space localization shown in Fig. 3 of the main text (positive-energy states from each chiral partner are shown in Fig. S5). An analogous mechanism is responsible for the emergence of three pairs of modes within the topological phase, with the corresponding positive-energy states shown for $t = 0$ and $t = 0.1$ in Fig. S5(c) and (f). Namely, the third pair emerges because of the third pair of the trench modes, which localize at the dislocation upon reconnecting the bonds. However, we do not show this explicitly as this chiral pair of the dislocation modes dissolves into the bulk already before the indirect gap closes.

## S3. FRAGILE DISLOCATION MODES IN THE OBSTRUCTED TOPOLOGICAL METAL

We here show the evolution of the number (Fig. S4) and the localization of the dislocation modes in terms of the local density of states (LDOS) on the lattice (Fig. S5) throughout the topological regime of the 2D SSH model [Eq. (S1)]. The LDOS of the most localized dislocation mode before the indirect bandgap closes is shown in Fig. 3 of the main text.

In Fig. S4, we first notice that the three chiral pairs of the dislocation modes for $t = 0$ are positioned within the gaps [Fig. S4(a)], while already for $t = 0.1$ two modes with highest absolute value of energy hybridize with the highest energy bands [Fig. S4(b)], and cease to exist as localized modes, which is corroborated by the evolution of the LDOS (only modes with positive energy are displayed) in Figs. S5(a)-(f). This hybridization occurs because the dislocation modes and the highest-energy bands transform under the same 1D irreps of the $C_{4v}$ group, $A_1$ and $B_2$. On the other hand, the two lower-energy pairs of modes in spite of entering the edge-band continuum [Fig. S4(c)-(e)],

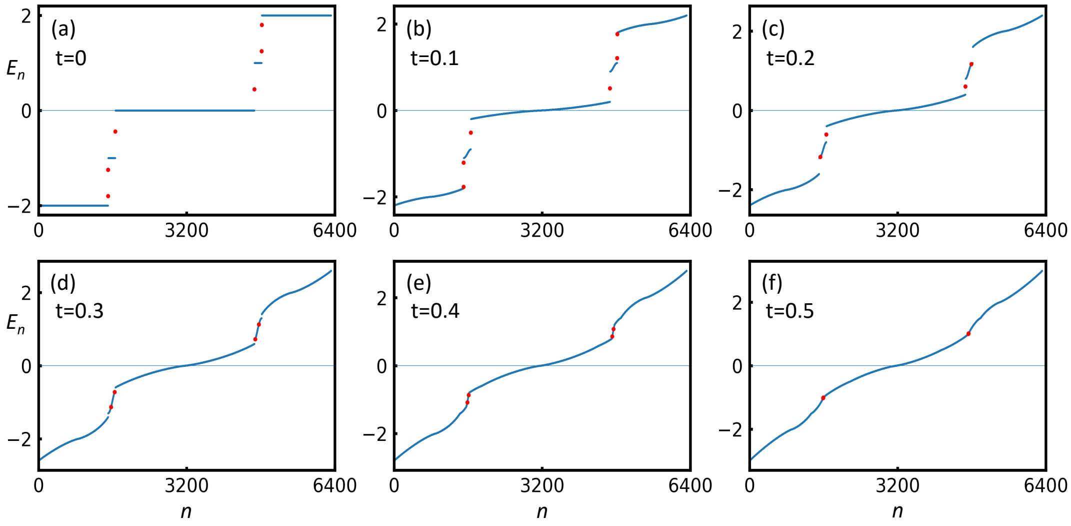


Figure S4. Evolution of the energy spectrum in the topological phase for the following values of the parameter $t$ in the Hamiltonian [Eq. (S1)]: (a) $t = 0$; (b) $t = 0.1$; (c) $t = 0.3$; (d) $t = 0.5$; (e) $t = 0.7$. We fix $\tau = 1$, the system size is $40 \times 40$ unit cells, and open boundary conditions are employed. Notice three chiral pairs of localized dislocation modes (marked in red) in (a) and (b). As the value of $t$ increases, the highest energy pair enters the high-energy bulk band and dissolves, so only the two remaining (protected) pairs are shown in (c)-(e).

remain localized [Figs. S5(g)-(l)]. Eventually, once the indirect bandgap closes for $t = 0.5$, see Fig. S4(f), these modes dissolve into the bulk continuum, as explicitly shown in Figs. S5(m) and (n). This is a consequence of the fact that both dislocation and the finite energy bulk modes transform under $A_1$ and $B_2$, therefore showing their fragility.

## S4. EVOLUTION OF THE CORNER MODES IN THE TOPOLOGICAL PHASE

In Fig. S6, we show the evolution of the localization in terms of the local density of states (LDOS) of a typical corner mode (one of the four corner-localized modes) as we sweep the topological phase of the 2D SSH model. The corner mode is well localized in the topological phase, with the localization approximately within a single unit cell, as we can see in Fig. S6(a)-(c). As the system approaches the indirect gap closing at $t = 0.5$, notice that the spectral weight of the corner mode significantly drops, Figs. S6(d)-(f), which is analogous to the behavior of the fragile dislocation modes in Fig. 3 of the main text. Here, the inter-unit-cell hopping is fixed $\tau = 1$.


[1] F. Liu and K. Wakabayashi, Phys. Rev. Lett. **118**, 076803 (2017).
[2] C. W. Groth, M. Wimmer, A. R. Akhmerov, and X. Waintal, New Journal of Physics **16**, 063065 (2014).
[3] W. A. Benalcazar and A. Cerjan, Phys. Rev. B **101**, 161116 (2020).
[4] B. Roy and V. Juričić, Phys. Rev. Res. **3**, 033107 (2021).

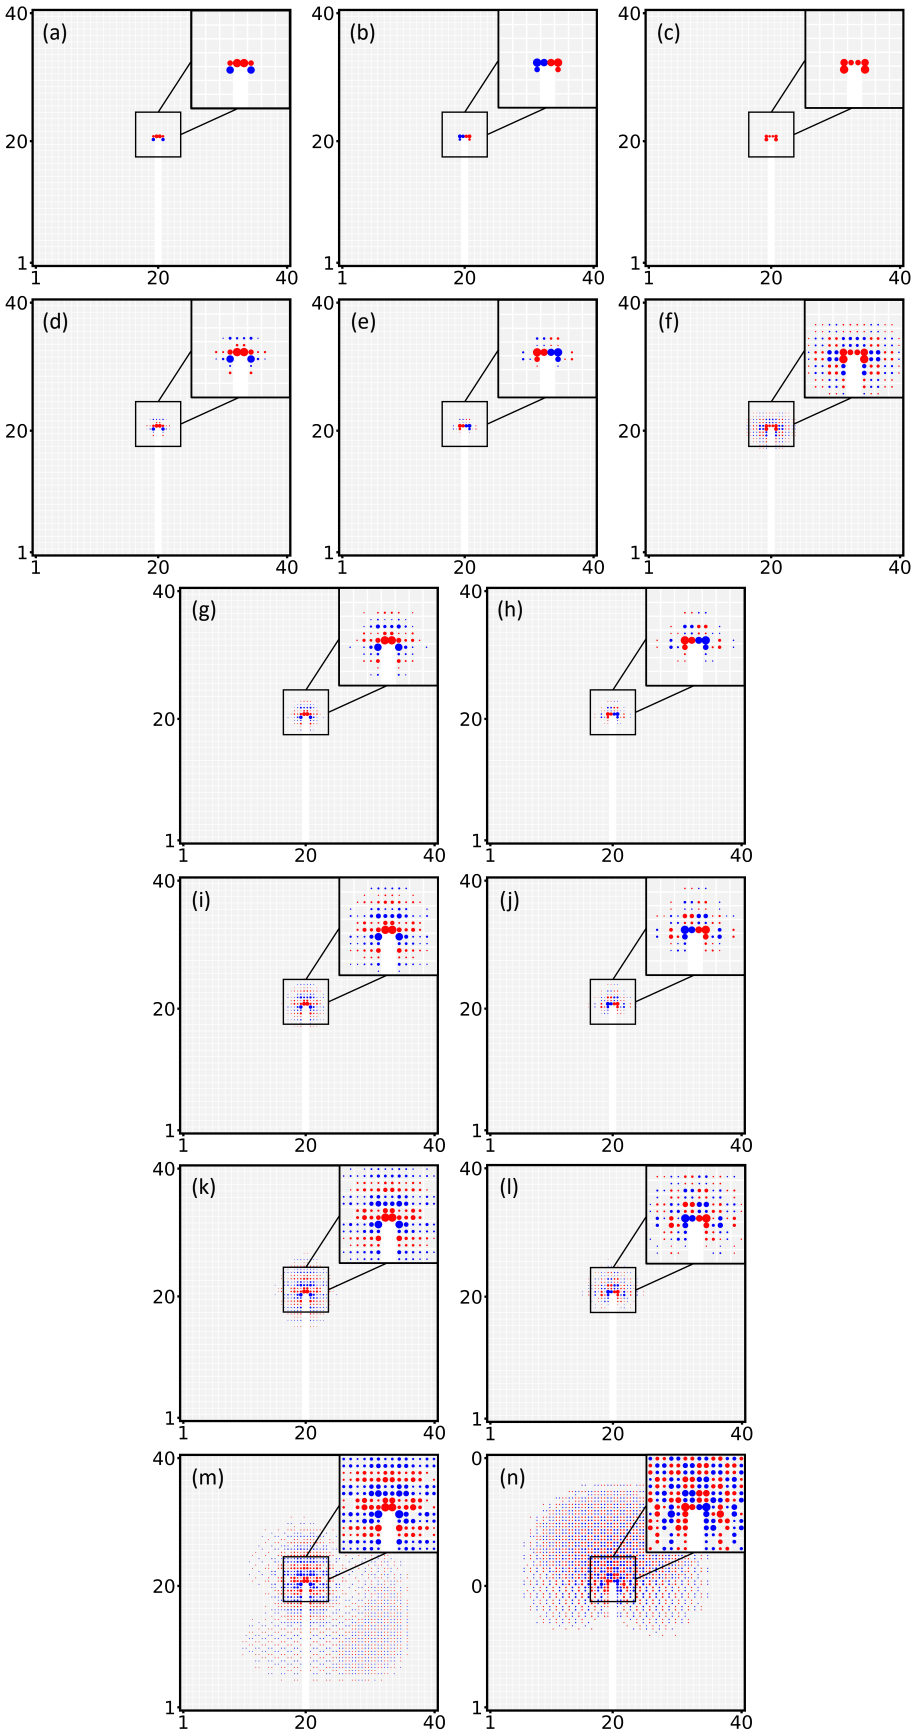


Figure S5. Positive-energy dislocation modes in the topological phase for different values of the intra-unit-cell hopping amplitude [Eq. (S1)]. (a)-(c) $t = 0$, (d)-(f) $t = 0.1$, (g)-(h) $t = 0.2$, (i)-(j) $t = 0.3$, (k)-(l) $t = 0.4$, (m)-(n) $t = 0.5$. We fix the value of the inter-unit-cell hopping $\tau = 1$. The system size is $40 \times 40$ unit cells, and open boundary conditions are employed.

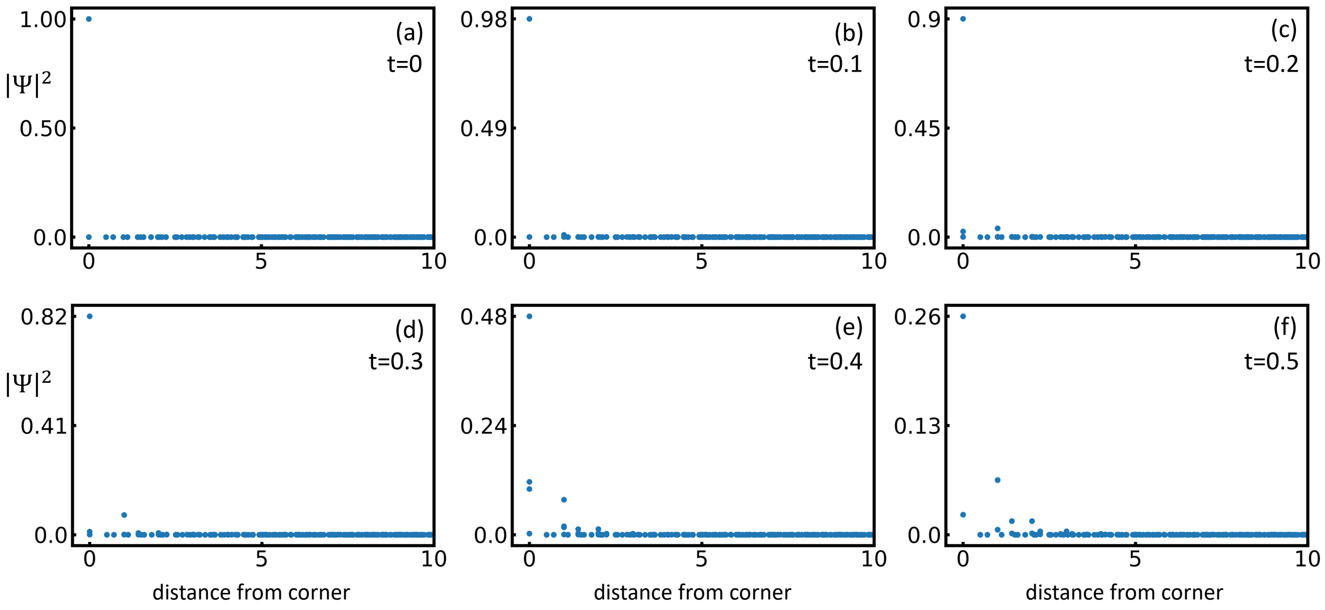


Figure S6. Evolution of the most localized corner mode in the topological phase. The local density of states (LDOS) of the mode is shown for the following values of the parameter $t$ in the Hamiltonian [Eq. (S1)]: (a) $t = 0$; (b) $t = 0.1$; (c) $t = 0.2$; (d) $t = 0.3$; (e) $t = 0.4$; (f) $t = 0.5$. We fix $\tau = 1$, the system size is $40 \times 40$ unit cells. The LDOS is shown only up to 10 lattice sites from the nearest corner since the LDOS farther away is negligible. The distance is given in units of the nearest-neighbor spacing, $a$.
